# Supplementary material for: Descending through a Crowded Valley - Benchmarking Deep Learning Optimizers
Source: arXiv:2007.01547 source file (2021-08-10)
Supplement: Supplementary file 1 [file standard_decay.tex]

\begin{tikzpicture}[baseline=(current bounding box.center),
  declare function={
    func(\x)= 1.0/((\x)^(.5))
   ;
  }
]
\begin{axis}[
  hide axis,
  axis background/.style={fill=TUgray!10},
  width=\figurewidth,height=\figureheight,
  ymin=-0.1, ymax=1.1,
  xmin=0, xmax=100,
  domain=0:100,samples=101,
]

\addplot [TUred,very thick] {func(x)};
\end{axis}
\end{tikzpicture}
